# Supplementary material for: Reinforcement Learning with Large Action Spaces for Neural Machine Translation
Source: arXiv:2210.03053 source file (2022-10-06)
Supplement: Supplementary file 1 [file appendix_x.tex]

% % This must be in the first 5 lines to tell arXiv to use pdfLaTeX, which is strongly recommended.
% \pdfoutput=1
% % In particular, the hyperref package requires pdfLaTeX in order to break URLs across lines.

% \documentclass[11pt, a4paper]{article}

% % Remove the "review" option to generate the final version.
% \usepackage[review]{acl}


% \usepackage{booktabs}
% \usepackage{graphicx}
% \usepackage{booktabs}
% % Standard package includes
% \usepackage{times}
% \usepackage{latexsym}
% \usepackage{graphicx}
% \usepackage{amsmath}
% \usepackage{caption}
% \renewcommand{\UrlFont}{\ttfamily\small}
% \usepackage{placeins} 
% \usepackage{stmaryrd}
% % For proper rendering and hyphenation of words containing Latin characters (including in bib files)
% \usepackage[T1]{fontenc}
% % For Vietnamese characters
% % \usepackage[T5]{fontenc}
% % See https://www.latex-project.org/help/documentation/encguide.pdf for other character sets

% % This assumes your files are encoded as UTF8
% \usepackage[utf8]{inputenc}

% % This is not strictly necessary, and may be commented out,
% % but it will improve the layout of the manuscript,
% % and will typically save some space.
% \usepackage{microtype}
% \usepackage{tikz}
% \usetikzlibrary{positioning}

% % If the title and author information does not fit in the area allocated, uncomment the following
% %
% %\setlength\titlebox{<dim>}
% %
% % and set <dim> to something 5cm or larger.

% \usepackage{amsthm}
% \usepackage{amssymb}
% \newtheorem{theorem}{Theorem}[section]
% \newtheorem{lemma}[theorem]{Lemma}

% \renewcommand\qedsymbol{$\blacksquare$}

%  \newcommand{\lc}[1]{\footnote{\color{cyan}Leshem: #1}}
%  \newcommand{\lcmod}[1]{{\color{cyan}#1}}
%  \newcommand{\oa}[1]{\footnote{\color{red}Omri: #1}}
%  %\newcommand{\oa}[1]{}
%  \newcommand{\oamod}[1]{{\color{red}#1}}
%  \newcommand{\as}[1]{\footnote{\color{magenta}Aviv: #1}}
%  \newcommand{\asmod}[1]{{\color{magenta}#1}}
%  \newcommand{\fix}{\marginpar{\color{orange}FIX}}
% \newcommand{\new}{\marginpar{\color{orange}NEW}}
% \setlength\marginparwidth{25pt}
% \newcommand\BibTeX{B\textsc{ib}\TeX}
% \graphicspath{{graphs/}}
% \begin{document}
%     \appendix


% \section{Computing Infrastructure}
% We train our models using 4 NVIDIA GTX Titan Black GPUs. The run time of the models varies between ten to twenty hours.

% \section{Methodology}\label{sec:data_sizes}
% % Please add the following required packages to your document preamble:
% % \paragraph{Architecture.}
% % \label{subsec:Arch.}
% % We use a similar setup as used by \citet{wieting2019beyond}, adapting their fairSeq-based \citep{ott2019fairseq} codebase to our purposes.\footnote{\url{https://github.com/jwieting/beyond-bleu}} Similar to their Transformer architecture we use gated convolutional encoders and decoders \citep{gehring2017convolutional}. We use 4 layers for the encoder and 3 for the decoder, the size of the hidden state is 768 for all layers, and the filter width of the kernels is 3. Additionally, the dimension of the BPE embeddings is set to 768.

% \paragraph{Optimization.}
% We optimize with Nesterov's accelerated gradient method
% \citep{sutskever2013importance} with a learning
% rate of 0.25, a momentum of 0.99, and
% re-normalize gradients to a 0.1 norm \citep{pascanu2012difficulty}.

% \paragraph{Data.}
% We use a the same data that used by \citet{wieting2019beyond}.
% For training data for cs-en, de-en, and ru-en,
% we use the WMT News Commentary v13\footnote{\url{ http://data.statmt.org/wmt18/translation-task}}
% \citep{bojar-etal-2017-findings} for training the models.
% Test sets are the official WMT18 test sets.
% For tr-en, we used for training the
% WMT 2018 parallel data, which consists of the
% SETIMES2 corpus \citep{Tiedemann2012ParallelDT}.
% The validation set is a concatenation of
% newsdev 2016 and 2017 released for WMT18. Our use of the data is aligned with the license and intended use of the data.

% \begin{table}[ht]
% %\resizebox{\columnwidth}{!}
% {%
% \begin{tabular}{@{}llll@{}}
% \toprule
% Lang. & Train   & Valid & Test                      \\ \midrule
% de-en & 284,246 & 6,003 & \multicolumn{1}{c}{2,998} \\
% cs-en & 218,384 & 6,004 & 2,983                     \\
% ru-em & 235,159 & 5,999 & 3,000                     \\
% tr-en & 207,678 & 6,007 & 3,000                     \\ \bottomrule
% \end{tabular}%
% }
% \caption{Number of sentence pairs in the training/validation/test sets for all four languages.}
% \end{table}

% \section{Entropy of STV and LTV}\label{sec:appendix_entropy_stv_ltv}
% As C19 suggested we can compare the peakiness of the two models by calculating the entropy of their distributions. Lower entropy indicates a more peaky distribution. We used KL divergence with respect to the uniform distribution in order to normalize the entropy and compare the peakiness of the two models. The STV model begins RL training with mean entropy of 0.300 and finishes with 0.269 while the 877 LTV begins with 0.258 and finishes with 0.264. This indicates that before RL training the LTV model was slightly more peaky than the STV, but after RL training they have similar peakiness.


% % \section{STV and LTV in small model}\label{sec:appendix_stv_ltv_small}
% % We also train STV and LTV models with inner dimension of size $d=256$. In this case, as we can see in figure \ref{fig:pro-shift-10-big-small_d256} the LTV is able to shift probability to the first place although STV is doing it more successfully. In addition, within the first one hundred ranks, STV reduces the probability of $88$ of them, whereas LTV only of $77$.  

% % % figure 1
% % \begin{figure}[ht]
% % \centering
% % \includegraphics[scale=0.28]{com_p_g_F.png}
% % \caption{Comparison of probability shift due to RL training of assign $y_{best}$ for ten first words for both LTV and STV with d=256. in green, you can see the results with BPE of size 1,000, STV. in blue are the results with BPE of size 30,000, LTV. a clear improvement of assigning $y_{best}$ in first place for STV.}
% % \label{fig:pro-shift-10-big-small_d256}
% % \end{figure}

% \section{Loading Bert embedding}\label{sec:appendix_bert_mle}
% We consider two options for initializing Bert embeddings for the MLE training, with and without freezing the embedding layer.
% The results were unequivocal, freezing the embedding layers has a very constructive effect on the results (table \ref{tab:table-bert-mle}). We estimate that freezing the embedding layers causes such a vast improvement in performance because it enables us to avoid the catastrophic forgetting of BERT parameters. Therefore, although using BERT embedding is helpful as initialization, by freezing the parameters we allow the model to better utilize BERT's embeddings.

% \begin{table}[ht]
% \centering
% \begin{tabular}{p{2.4cm}|p{0.9cm}|p{0.9cm}|p{0.9cm}|p{0.9cm}}
% %{@{}lllll@{}}
% \toprule
% Model & de-en & cs-en & ru-en & tr-en \\ \midrule
% MLE                  & 22.38 & 15.81 & 17.31 & 12.60 \\
% MLE+Bert W/o freeze  & 22.99    & 15.32 & 17.57 & 12.65\\
% MLE+Bert with freeze &   23.46  & 16.59   & 18.14 & 14.15\\
% diff.                & 0.47  & 1.27 & 0.57 & 1.50  \\
%  \bottomrule
% \end{tabular}
% \caption{\label{tab:table-bert-mle} Comparison of MLE models with BERT embedding with and without freezing.}
% \end{table}


% \section{Number of parameters}\label{sec:appendix_pram}
% In Table \ref{tab:table-bert-pram-comp} we provide a comparison of the number of trainable parameters with and without freezing the embedding layer.
% %in two settings, one when we are freezing the embedding layer and the second when we don't freeze.
    
% % \begin{table}[ht]
% % \begin{tabular}{@{}lllll@{}}
% % \toprule
% % \# parameters & de-en & cs-en & ru-en & tr-en \\ \midrule
% % Freeze        & 11.9M & 11.6M & 11.1M & 11.6M \\
% % W/o freeze    & 22.7M & 21.1M & 19.8M & 22.5M \\
% % Ratio         & 0.52  & 0.54  & 0.56  & 0.51  \\ \bottomrule
% % \end{tabular}

% % \caption{\label{tab:table-reg-pram-comp} Comparison if trainable parameters in large bpe setting.}
% % \end{table}

% % table 4:
% \begin{table}[ht]
% \centering
% \begin{tabular}{@{}lllll@{}}
% \toprule
% \# parameters & de-en & cs-en & ru-en & tr-en \\ \midrule
% Freeze & 30.2M      &  29.3M     &   27.9M    &  29.4M     \\ 
% W/o Freeze      &  77.2M     &   76.2M   &   74.8M    &   76.4M    \\ 
% Ratio &  0.39     &   0.38    & 0.37      &  0.38  \\  \bottomrule
% \end{tabular}
% \caption{\label{tab:table-bert-pram-comp} Comparison if trainable parameters.}
% \end{table}

% % \section{Medium Size Data Experiment}\label{sec:m_exp}
% % For those experiments, we use English-German data containing $2,826,714$ sentences (WMT Dataset after some filtering). We conduct the experiments with both proposed methods. The results of the first method where we reduce the target vocabulary size are on table \ref{tab:mid_stv_ltv}. Results indicate that indeed smaller action space enable better generalization even in medium-size data scenarios. 


% % % table 4:
% % \begin{table}[ht]
% % \centering
% % \begin{tabular}{@{}lllll@{}}
% %  \toprule
% %  Model & de-en \\
% %  \midrule
% %  LTV  & 31.10   \\
% %  LTV+RL&   32.44 \\
% %  Diff. & 1.34 \\
% %  \midrule
% %  STV  & 41.55  \\
% %  STV+RL&   43.35 \\
% %  Diff. & 1.80\\ \bottomrule
% % \end{tabular}
% % \caption{\label{tab:mid_stv_ltv} BLEU score of STV and LTV with medium size data. Results indicating that the method is helpful in medium size data setting as well}
% % \end{table}

% % In the second method, we aim to implicitly reduce the effective action space size by incorporating informative target embedding and freezing it. Results in table \ref{tab:mid_bert} show that the MLE result without BERT is higher than the results with BERT. This is not surprising as a better embedding matrix can be learned when more data is available. Although this observation, ruining the experiment described in \S 7 shows similar results to the embedding learned with a small amount of data. Regarding the effect of the RL training with informative target embedding, it seems that there is a relative gain to $+BERT+RL$ over $+RL$. Regarding freezing, when combine with basic $+RL$ led to inferior improvement of $2.98$ BLEU points and together with $+BERT+RL$ gain $2.63$ BLEU points over $+BERT$. These results show that freezing the target embedding when more data is available can lead to lesser results. The cause for this can be the change in the model capacity. Overall, it seems that our proposed method has some differences when moving to medium resources scenario but the core idea that RL training benefit from small action space and that informative target embedding is important remains.

% % % table 5:
% % \begin{table}
% % %\large
% % % \resizebox{\columnwidth}{!}
% % \centering
% % {\begin{tabular}{@{}lllll@{}}
% % \toprule
% % MODEL           & de-en  \\ \midrule
% % MLE             & 29.62  \\
% % +RL             & 32.75  \\
% % % \midrule
% % Diff.      & 3.13  \\
% % \midrule
% % +BERT           & 28.39  \\
% % +BERT+RL       & 31.92  \\
% % Diff. & 3.53  \\ \bottomrule
% % \end{tabular}
% % }\caption{\label{tab:mid_bert}  BLEU score of second method with medium size data. Results showing that the improvement of RL when using BERT's target embedding is bigger then the baseline. Nevertheless, the MLE model with BERT gain inferior results. This can be a results of the ability of the model to learn somewhat good embedding from the data signal when it is big enough}
% % \end{table}

% \section{Formalizing the intuition behind freezing the embedding layer}\label{sec:appendix_proof}
% Here we want to formalize the intuition behind freezing the embedding layer. We explicitly calculate the gradients of the cross-entropy (CE) loss of the one-hot vector, $y$, and the distribution vector, $\hat y$ of the model $f_{\theta} = h_{\theta_{2}} \circ g_{\theta_{1}}$ output (henceforth, we will discard the parameters notation from $f,g$ and $h$). We will discuss two cases, one when we freeze $\theta_{2}$ and the second when we are not. We note that $\theta_{2} \in \mathbb{R}^{d\times |V_{T}|}$ is the embedding layer where each row, $\rho_i$, is the representation of the $k$’s word in the vocabulary. Moreover, $h: \mathbb{R}^d \rightarrow \mathbb{R}^{|V_{T}|}$ is the function defined by multiplying the output of $g$, denoted by $v \in \mathbb{R}^d$, by $\theta_{2}$, and then taking the soft-max of the output vector, hence $\forall k\in |V_{T}|;  h_k(v) = \frac{exp(\rho_k \cdot v)}{\sum_l exp(\rho_l\cdot v)}$. Therefore assigning to each word some probability, $\hat y_k$, to be the next one in the sentence.

% %Similarly, we can define the scalar function $\forall k\in |V_{T}|; f_k: \mathbb{R}^d \rightarrow \mathbb{R}$ that get as an input source sentence, $X$, prefix of the translation, $y_{<i}$, and defined by parameters, $\theta$, and output the probability of the next token to be the $k$’s word in vocabulary. To be more precise, the input of $f_k$ is a vector $p \in \mathbb{R}^d$ that represent $X$ and $y_{<i}$ in the inner dimension of the net. In this terminology, the model chooses the next token to be the one that corresponding to the $f_k$ that upon the input $p$ return the biggest probability. Then we calculating the CE loss between the model distribution and the one hot vector encoding of the gold token, and updating the model parameters according to the gradient of CE.

% Now, we want to investigate the update defined by the gradients of the CE loss in the setting when two words, $w_1$ and $w_2$ have the same representation, $\rho_1 = \rho_2$. We consider the case where one of them is the gold token, w.l.g. $w_1$. We note this case by $\Big|^1$.
% %In this setting we want to compare the gradients when the model choose $x_1$ to when the model choose $x_2$, corresponding with two input vectors $p_1$ and $p_2$. 
% % respectfully, for two input points $p_1$ and $p_2$. 
% %reflecting that both of them suit the context and have similar meaning.

% We turn to examine the gradient in this setting for both cases. We start by realizing that if all the partial derivatives of the CE loss, $L$, exist then the gradient is the vector of all the partial derivatives meaning, $\nabla_{\theta}L=\begin{pmatrix} \nabla_{\theta_1}L \\ \nabla_{\theta_2}L \end{pmatrix}$ 
% and we can separate the calculation into two parts, one with respect to $\theta_1$ and the second with respect to $\theta_2$. 

% By definition, in the case where we freeze $\theta_2$ we will keep $\rho_1$ and $\rho_2$ the same. We will now show that in the case when we don't freeze $\theta_2$ the update will be different.
% % introduce notation $f(r:\theta, y_{<i}, z)$ where z encoder output (maybe the same to put x, r the input vector for the decoder. for one input we get $x_1$ for another $x_2$.


% \begin{lemma}
% If $\theta_2$ is not frozen then:
% %$\nabla_{\theta_2}L\Big|_{p_1} \neq \nabla_{\theta_2}L\Big|_{p_2}$. specifically, 
% Updates are differe: $\Delta\rho_1!=\Delta\rho_2$.
% %consequentially, we  
% % we update $\rho_1$ differently from $\rho_2$ upon our choose. 
% \end{lemma}

% \begin{proof}
% We start by noticing that multiplying $v$ by $\theta_2$ is a linear transformation so for points $p_1$ and $p_2$ we will get the same derivative as $\rho_1 = \rho_2$, moreover by taking the soft-max of those identical outputs we will get the same outputs. Hence, we get that $\forall i\in [d];  \frac{\partial \hat y_1}{\partial v_i} = \frac{\partial \hat y_2}{\partial v_i}$, similarly $\frac{\partial \hat y_1}{\partial \rho_{1i}} = \frac{\partial \hat y_2}{\partial  \rho_{2i}}$. 

% We continue by calculating the derivative of the CE. 
% The CE loss is defined by:
% \begin{equation}
%     L(y, \hat y) = \sum_i y_i log(\hat y_i)
% \end{equation}
% The derivative is: $\frac{\partial L}{\partial \hat y_i}= \sum_i y_i \frac{1}{\hat y_i}$ we notice that  $y$ is a one hot vector i.e., $y_1=1$ and $\forall i\in [2,|V_{T}|]; y_i = 0$. Therefore, the derivative will be different from $i=1$ to all other $i$'s. Specifically, $\forall i\in [d]; \frac{\partial L}{\partial \rho_{1i}} \neq \frac{\partial L}{\partial \rho_{2i}}$ .
% Putting it all together we get:
% \begin{equation}
%     \frac{\partial L}{\partial \rho_{1i}} = \frac{\partial L}{\partial \hat y_1} \cdot \frac{\partial \hat y_1}{\partial \rho_{1i}} \neq \frac{\partial L}{\partial \hat y_2} \cdot \frac{\partial \hat y_2}{\partial \rho_{2i}} = \frac{\partial L}{\partial \rho_{2i}}
% \end{equation}
% Proving that $\rho_1$ and $\rho_2$ updates are different.

% \end{proof}


% \begin{lemma}
% For both cases, the update of $\theta_1$ is symmetric to the gold being $w_1$ or $w_2$. 
% %$\nabla_{\theta_1}L = \nabla_{\theta_1}L$ meaning, the update of $\theta_1$ we 
% $\nabla_{\theta_2}L\Big|^1 = \nabla_{\theta_2}L\Big|^2$.
% %$\nabla_{\theta_1}f$ is the same regardless of model choosing $x_1$ or $x_2$.
% \end{lemma}

% \begin{proof}
% Given a parameter $\lambda \in \theta_1$, we inspect the derivative of $L$ with respect to $\lambda$. We use here Einstein summation notation.
% \begin{equation}
%     \frac{\partial L}{\partial \lambda}\Big|^1 = \frac{\partial L}{\partial v_i} \cdot \frac{\partial v_i}{\partial \lambda}\Big|^1 = \frac{\partial L}{\partial v_i} \cdot \frac{\partial v_i}{\partial \lambda}\Big|^2 = \frac{\partial L}{\partial \lambda}\Big|^2
% \end{equation}
% We deduce $\frac{\partial v_i}{\partial \lambda}\Big|^1 = \frac{\partial v_i}{\partial \lambda}\Big|^2$, as the derivative of $v_i$ is independent of the question which word is the gold.
% In order to justify the second equality we used, we will write the derivative of $L$ with respect to $v_i$.
% \begin{equation}
%     \frac{\partial L}{\partial v_i}\Big|^1 = \frac{\partial L}{\partial \hat y_k} \cdot \frac{\partial \hat y_k}{\partial v_i}
% \end{equation}
% Clearly, we only need to check the elements that change by switching the gold from being $w_1$ to $w_2$ or vice versa. Therefor all the second terms that multiply by $\frac{\partial L}{\partial \hat y_k}$ for $k\in [3,|V_{T}|]$ didn’t change. We already proved that $\forall i\in [d];  \frac{\partial \hat y_1}{\partial v_i} = \frac{\partial \hat y_2}{\partial v_i}$ 
% %what translated here to $\frac{\partial \hat y_1}{\partial \rho_{1j}} \cdot \frac{\partial \rho_{1j}}{\partial v_i} = \frac{\partial \hat y_2}{\partial \rho_{2j}} \cdot \frac{\partial \rho_{2j}}{\partial v_i}$. 
% Finally, because we switch the gold, $\frac{\partial L}{\partial \hat y_1}$ and $\frac{\partial L}{\partial \hat y_2}$ indeed switch there values but both of them are multiply by the same values as $\frac{\partial \hat y_1}{\partial v_i} = \frac{\partial \hat y_2}{\partial v_i}$. Overall, the derivative is unchanged.
% \end{proof}

% To conclude, in the motivational setting we discussed, when we freeze $\theta_2$ we keep semantically close vectors unchanged while if we don't freeze $\theta_2$ we enable them to change. As consequence, in further steps, this change will affect on $\theta_1$ also. In a similar manner, as long as the representation is similar, all layers but the penultimate would update both words similarly.

% % We can calculate $\nabla_{\theta}f=
% % \begin{pmatrix}
% % \nabla_{\theta_1}f \\ \nabla_{\theta_2}f 
% % \end{pmatrix}$ as all partial derivatives of $f$ exist.
% % because all partial derivatives of a function exist  


% % Denote the function that the network computes with $f_{\theta}$.
% % $f_{\theta}$ can be written as $h_{\theta_{2}} \circ g_{\theta_{1}}$,
% % where $\theta = \left( \theta_{1}, \theta_{2} \right)$, $g$ maps the input -- source sentence $X$
% % and model translation prefix $y'_{<i}$ -- into $\mathbb{R}^d$, and $h$ maps $g$’s output into $\mathbb{R}^{|V_{T}|}$.

% \section{Semantic scores for the second method}\label{sec:appendix_bert_sim}

% % % table 1:
% % \begin{table}[ht]
% % \centering
% % \begin{tabular}{ @{}lrrrr@{}  }
% %  \toprule
% %  Model & de-en & cs-en &ru-en& tr-en\\
% %  \midrule
% %  LTV  & 80.09    & 74.48 & 78.17 & 69.32\\
% %  LTV+RL&   80.84  & 75.45   & 79.42 & 69.93\\
% %  Diff. & 0.75 & 0.97 &  1.25 & 0.61\\
% %  \midrule
% %  STV  & 98.95    & 98.64 & 98.97 & 98.45\\
% %  STV+RL&   99.07  & 98.68   & 99.01 & 98.55\\
% %  Diff. & 0.12 & 0.04 &  0.04 & 0.10\\

% %  \bottomrule
% % \end{tabular}
% % \caption{\label{tab:table-small-big-results} SIM scores}
% % \end{table}

% % table 1:
% % \begin{table}[ht]
% % \centering
% % \begin{tabular}{ @{}lrrrr@{}  }
% %  \toprule
% %  Model & de-en & cs-en &ru-en& tr-en\\
% %  \midrule
% %  LTV  & 75.87    & 70.55 & 73.57 & 65.19\\
% %  LTV+RL&   76.89  & 71.50   & 74.96 & 65.82\\
% %  Diff. & 1.02 & 0.95 &  1.39 & 0.63\\
% %  \midrule
% %  STV  & 93.54    & 92.92 & 92.43 & 91.50\\
% %  STV+RL&   94.50  & 93.57   & 93.23 & 93.13\\
% %  Diff. & 0.96 & 0.65 &  0.80 & 1.63\\

% %  \bottomrule
% % \end{tabular}
% % \caption{\label{tab:table-small-big-results} smaile scores}
% % \end{table}

% %We present the SIM results for the second method. SIM is a measure of semantic similarity that assigns partial credit to semantically correct but lexically different translations \citep{wieting2019beyond}.
% Our method of freezing informative initialization of the embedding layer aims to generalize across different but semantically close actions. In order to test the ability of our model to generalize we used SIM. SIM is a measure of semantic similarity that assigns partial credit to semantically correct but lexically different translations \citep{wieting2019beyond}.
% %As our second method aims to generalize across different but semantically close actions, this score function can reflect this ability.
% Table \ref{tab:table-BERT-sim-results} shows our model results and exhibits similar trends to the BLEU scours. Here we see even greater gains for cs-en and ru-en languages pairs. Those results may indicate that the model was able to predict tokens that are semantically close to the gold token.

% \begin{table}[ht]
% \large
% \resizebox{\columnwidth}{!}{%
% \begin{tabular}{@{}lllll@{}}
% \toprule
% MODEL           & de-en & cs-en & ru-en & tr-en \\ \midrule
% MLE             & 70.03 & 63.29 & 66.17 & 59.68 \\
% +RL             & 71.17 & 63.29 & 66.17 & 59.99 \\
% % \hline
% \midrule

% % \hline
% % \hline
% +RL+FREEZE      & 71.03 & 64.29 & 66.66 & 60.52 \\
% % \midrule
% +BERT          & 71.56 & 64.26 & 66.70 & 61.75 \\
% +BERT+RL       & 72.44 & 65.80 & \textbf{67.94} & \textbf{63.59} \\
% +BERT+RL+FREEZE & \textbf{72.81} & \textbf{66.44} & 67.66 & \textbf{63.59} \\ \bottomrule
% \end{tabular}%
% }\caption{\label{tab:table-BERT-sim-results}SIM scores on translating four languages to English.}
% \end{table}

% % \begin{table}
% % \large
% % \resizebox{\columnwidth}{!}{%
% % \begin{tabular}{@{}lllll@{}}
% % \toprule
% % MODEL           & de-en & cs-en & ru-en & tr-en \\ \midrule
% % MLE             & 66.84 & 60.20 & 62.97 & 56.25 \\
% % +RL             & 68.37 & 60.20 & 62.97 & 56.82 \\
% % % \hline
% % \midrule

% % % \hline
% % % \hline
% % +RL+FREEZE      & 68.24 & 61.44 & 63.50 & 57.38 \\
% % % \midrule
% % +BERT           & 68.57 & 61.46 & 63.42 & 58.28 \\
% % +BERT+RL       & 69.54 & 64.80 & \textbf{75.05} & 60.28 \\
% % +BERT+RL+FREEZE & \textbf{69.92} & \textbf{72.78} & 64.40 & \textbf{60.28} \\ \bottomrule
% % \end{tabular}%
% % }\caption{\label{tab:table-BERT-results}smile}
% % \end{table}

% \section{Human Evaluation Information} \label{sec:human_eval_info}
% We recruited the service of two professional translators via translations providers.
% \subsection{Human Evaluation Instructions}
% You will be shown:

% \begin{enumerate}
%     \item An English segment of text;
%     \item Corresponding translation into English.
% \end{enumerate}

% There are three parts to each annotation:
% \begin{enumerate}
%     \item Read the English segment;
%     \item Read the translation and compare its meaning to the meaning of the original English segment;
%     \item Give a score between 0-100 describing how close the meaning of the translation is to the meaning of the original English segment.
% \end{enumerate}

% \bibliography{anthology,custom}
% \bibliographystyle{acl_natbib}
% \end{document}
